# Supplementary material for: Statistical modeling of quantum error propagation
Source: arXiv:2408.15459 source file (2024-08-28)
Supplement: Supplementary file 1 [file appendix.tex]

\section{Appendix}

\begin{table}[h!]
    \centering
    \begin{tabular}{|c|c|c|c|c|c|c|}
        \hline
        Index & $Q_1[1]$ & $Q_1[2]$  & $Q_3[1]$ & $Q_3[2]$ & $\#$ Errors in  $Q_1[3],Q_2[3]$ & Probability \\ \hline
        1 &  0 &  0 &  0 &  0& 0 &  $(1-p)^4$\\ \hline
        2 &  0 &  0 &  0 &  1& 1 &  $p(1-p)^3$\\ \hline
        3 &  0 &  0 &  1 &  0& 1 &  $p(1-p)^3$\\ \hline
        4 &  0 &  0 &  1 &  1& 0 &  $p^2(1-p)^2$\\ \hline
        5 &  0 &  1 &  0 &  0& 1 &  $p(1-p)^3$\\ \hline
        6 &  0 &  1 &  0 &  1& 2 &  $p^2(1-p)^2$\\ \hline
        7 &  0 &  1 &  1 &  0& 2 &  $p^2(1-p)^2$\\ \hline
        8 &  0 &  1 &  1 &  1& 1 &  $p^3(1-p)$\\ \hline
        9 &  1 &  0 &  0 &  0& 2 &  $p(1-p)^3$\\ \hline
        10 & 1 &  0 &  0 &  1& 1 &  $p^2(1-p)^2$\\ \hline
        11 & 1 &  0 &  1 &  0& 1 &  $p^2(1-p)^2$\\ \hline
        12 & 1 &  0 &  1 &  1& 2 &  $p^3(1-p)$\\ \hline
        13 & 1 &  1 &  0 &  0& 1 &  $p^2(1-p)^2$\\ \hline
        14 & 1 &  1 &  0 &  1& 0 &  $p^3(1-p)$\\ \hline
        15 & 1 &  1 &  1 &  0& 0 &  $p^3(1-p)$\\ \hline
        16 & 1 &  1 &  1 &  1& 1 &  $p^4$\\ \hline

    \end{tabular}
    \caption{All $16$ cases for the }
    \label{tab:transversal}
\end{table}
